# Supplementary material for: Experimental observation of one-dimensional superradiance lattices in ultracold atoms
Source: arXiv:1805.07965 source file (2018-05-21)
Supplement: Supplementary file 1 [file SI-2018.pdf]

# Supplementary Material for "Experimental observation of one-dimensional superradiance lattices in ultracold atoms"

Liangchao Chen,[1,2] Pengjun Wang*,[1,2] Zengming Meng,[1,2] Lianghui Huang,[1,2] Han Cai†,[3,4] Da-Wei Wang,[3,4] Shi-Yao Zhu,[3,5] and Jing Zhang‡[1,5]

[1]*State Key Laboratory of Quantum Optics and Quantum Optics Devices, Institute of Opto-Electronics, Shanxi University, Taiyuan 030006, P.R.China*

[2]*Collaborative Innovation Center of Extreme Optics, Shanxi University, Taiyuan 030006, P.R.China*

[3]*Interdisciplinary Center of Quantum Information and Department of Physics, Zhejiang University, Hangzhou 310027, P.R.China*

[4]*Institute of Quantum Science and Engineering, Texas A&M University, College Station, TX 77843, US*

[5]*Synergetic Innovation Center of Quantum Information and Quantum Physics, University of Science and Technology of China, Hefei, Anhui 230026, P. R. China*

## THE EXPERIMENTAL SET-UP

Two independent grating feedback external cavity diode lasers (ECDLs) are used to generate the coupling and probe laser beams. One of ECDLs for the coupling fields serves as the master laser and is frequency-locked by the saturated absorption spectroscopy to the D1 line of $^{87}$Rb. A double-pass acousto-optic modulator (AOM) (3200-124, Crystal Technology, Inc) with a frequency shift $+110\times2$ MHz is used in the saturated absorption spectroscopy. The frequency of the master laser is locked with a detuning $+110$ MHz from the transition $|e\rangle = |F' = 1, m'_F = 1\rangle$ and $|m\rangle = |F = 1, m_F = 1\rangle$. The master laser output is coupled into a polarization maintaining single-mode fibre in order to improve the stability of the beam direction and the beam-profile. After the fibre, the laser is sent through a single-pass AOM (AOM2) and the frequency is shifted by $-110$ MHz. Therefore, this laser is resonant with the transition between $|e\rangle$ and $|m\rangle$. In the experiment, the intensity and frequency of the coupling laser are controlled by AOM2.

Another ECDL for the probe light serves as the slave laser and is locked to the master laser by the optical phase-locked loop. The frequency of the slave laser is in the vicinity of the $^{87}$Rb D1 line transition between $|g\rangle \equiv |F = 2, m_F = 2\rangle$ and $|e\rangle$. The phase lock loop is designed as following. The master and slave lasers are superimposed and measured by an ultrafast detector, which shows a beating signal with a frequency around 6835 MHz. The beating signal and another reference signal (36 MHz) are passed to a phase frequency detector (PFD). The PFD produces an error feedback signal. The slowly varying part of the error feedback signal is added into the piezoelectric ceramic of the slave laser, while the fast part is added to the current modulation of the slave laser. Once locked, the linewidth of the frequency difference between the master and slave lasers is reduced to several Hz. In the experiment of measuring the superradiance signal, we change the frequency of the probe beam by setting the locked frequency point of the PFD.

A superradiance signal detected by the EMCCD is shown in Fig. S1. The finite size of the spot demonstrates the directionality of the superradiance.

## THEORETICAL MODEL

A two-level system with states $|e\rangle$ and $|m\rangle$ coupled by a standing wave has two important parameters, the Rabi frequency $\Omega=\mu E/\hbar$ with $E$ the electric field amplitude of the coupling laser and $\mu$ the transition dipole moment, the single photon recoil energy $E_r = \hbar^2 Q^2/2m$ where $\hbar Q = 2\pi\hbar/\lambda_0$ is the single photon recoil momentum and $\lambda_0$ is the atomic transition wavelength. The Hamiltonian includes two parts, $H = K + V$, where $K = \hbar^2 k^2/2m$ is the recoil energy and $V = 2\Omega\cos Qx\,|e\rangle\langle m| + h.c.$ is the interaction Hamiltonian. From simplicity, the momentum is denoted in unit of $Q$. Due to the spatial periodicity of the coupling fields, the Hamiltonian can be written in the discrete plane

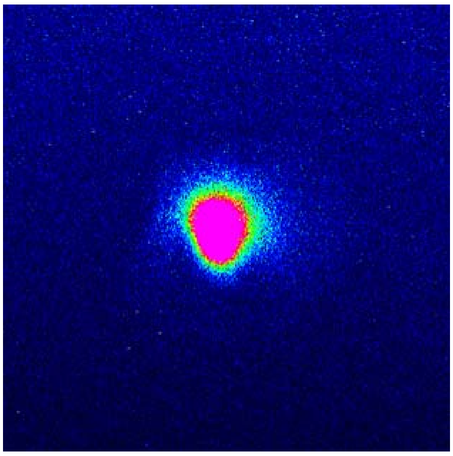

FIG. S1: **Image of the superradiance signal detected on EMCCD.**

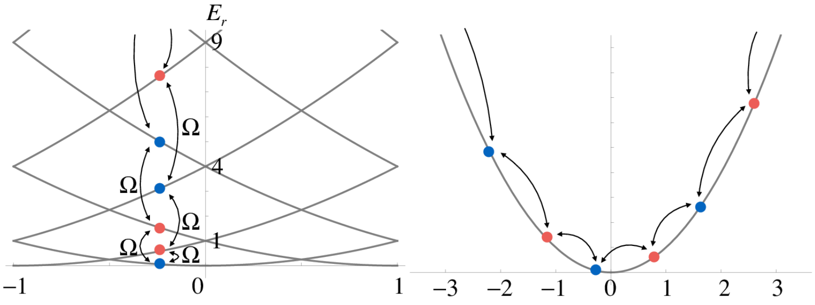


FIG. S2: (a) Solid lines show the free particle dispersion relation. For $k = -0.25$, states with opposite spin (atomic state) couple with each other, where blue (red) dots denote $|m\rangle(|e\rangle)$ atomic state. (b) The equivalent model, a TB lattice in the background of a harmonic potential for $k = -0.25$ in Fig.1a.

wave basis of $|k+2n\rangle_m$ and $|k+(2n+1)\rangle_e$ where $n$ is an integer,

$$H = \Psi^+ \begin{pmatrix} \cdots & \Omega & & & & & \\ \Omega & E_r(k-2)^2 & \Omega & & & & \\ & \Omega & E_r(k-1)^2 & \Omega & & & \\ & & \Omega & E_r k^2 & \Omega & & \\ & & & \Omega & E_r(k+1)^2 & \Omega & \\ & & & & \Omega & E_r(k+2)^2 & \Omega \\ & & & & & \Omega & \cdots \end{pmatrix} \Psi, \tag{S1}$$

where $\Psi^\dagger = (\ldots |k-2\rangle_m, |k-1\rangle_e, |k\rangle_m, |k+1\rangle_e, |k+2\rangle_m, \ldots)$

This Hamiltonian is for a one-dimensional tight-binding (TB) lattice in momentum space with a lattice constant $2Q$, a nearest neighbor hopping amplitude $\Omega$, and a harmonic potential $E_r k^2$. Compared with real space lattices, the potential energy and kinetic energy exchange their roles [S1] in a momentum space lattice. The real space potential energy $V$ contributes to the hopping term in a momentum space lattice, while the real space kinetic energy $\hbar^2 k^2/2m$ contributes to a harmonic potential, as shown in Fig.S2.

### Subrecoil coupling regime $\Omega < E_r$

The eigenstates of the spatially periodic Hamiltonian are Bloch wavefunctions of which the lattice momenta $k$ being good quantum numbers. For the momenta at the boundary of the first Brillouin zone, $k = \pm 0.5$, $|k\rangle_m$ and $|k \mp 1\rangle_e$

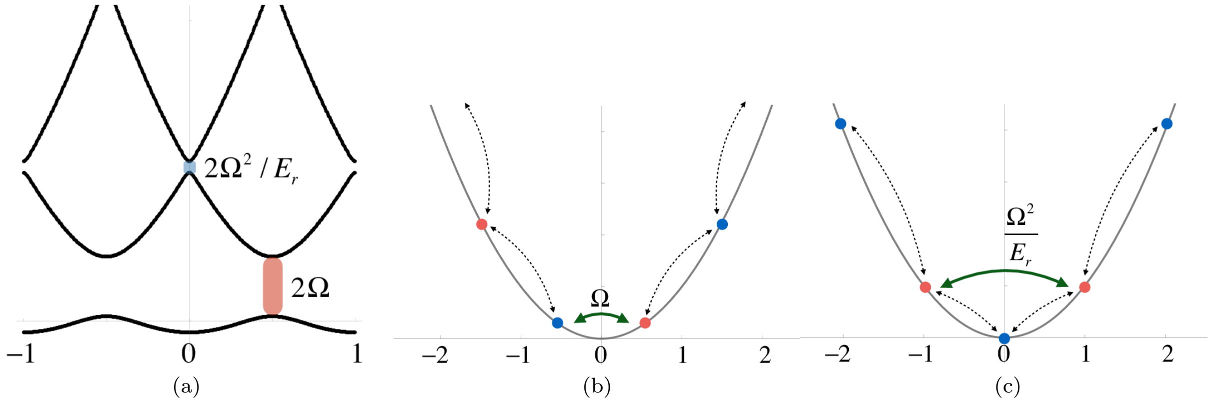


FIG. S3: (a) The band structure of the TB lattice for $\Omega = 0.2E_r$. (b) The TB model when $k = 0.5$ is shown. Sold and dash lines denote the on-resonant and off-resonant coupling between $|k\rangle_m$ and $|k-1\rangle_e$. (c) The TB model when $k = 0$ is shown.

has the same energy, as shown in Fig.S3b, and the model can be simplified to a two-level system. The effective Hamiltonian can be written as

$$H = \hat{\sigma} \cdot \mathbf{B} + \frac{E_r}{4}\mathbf{I}, \tag{S2}$$

where $\mathbf{B} = (\Omega, 0, -E_r k)$, $\hat{\sigma}$ is the spin operator of $|\uparrow\rangle = |k-1\rangle_e$ and $|\downarrow\rangle = |k\rangle_m$. We could observe spin oscillations [S2, S3] and the 1st order atomic Bragg scattering [S4] when atom is pumped into this two-level system. A second-order coupling strength opens the gap near $k = 0$ between the second and third bands, where the effective coupling between $|k-1\rangle_e$ and $|k+1\rangle_e$is $V_{2nd} =_e \langle k-1| V \frac{1}{E_e - E_m} V |k+1\rangle_e = \frac{\Omega^2}{E_r}$, as shown in Fig.S3c. The 2nd order Bragg scattering could be observed [S4]. In this subrecoil regime, i.e., $\Omega < E_r$ we could always treat the system as an effective two-level system decoupled from other states at the momenta where gaps open. The experiments on atom laser, atom interferometry and spin-orbit coupling are mostly done in this subrecoil regime.

### Superrecoil coupling regime $\Omega \gg E_r$

In the regime of $\Omega \gg E_r$, which is the case in our experiment, we define a length scale $\eta = \sqrt{\Omega/E_r}$ within which the potential energy is negligible compared with the hopping energy. The states inside this length form a tight-binding lattice structure in momentum space [S5]. The real space kinetic energy is a shallow parabolic potential background in momentum space [S6, S7]. It is reasonable to neglect the shallow harmonic potential in our experiment considering the finite decay rate and the large $\eta \approx 100$. After the atom is pumped into the lattice, the number of sites it can hop before decaying is $\Omega/\Gamma$. If this number is much smaller than $\eta$, we can neglect the effect of the harmonic potential. This requires $\Gamma \gg \sqrt{\Omega E_r}$, which is satisfied in our experiment.

## HAMILTONIAN

The Hamiltonian of the BEC atoms interacting with the probe and coupling light beams is (with $\hbar = 1$),

$$\begin{aligned} H &= \int d\mathbf{q}(-\Delta_p + \frac{\hbar^2 k^2}{2m})b_e^\dagger(\mathbf{q})b_e(\mathbf{q}) + (-\Delta_{2\text{ph}} + \frac{\hbar^2 k^2}{2m})b_m^\dagger(\mathbf{k})b_m(\mathbf{k}) \\ &+ \Omega_1 b_e^\dagger(\mathbf{q})b_m(\mathbf{q}-\mathbf{k}_1) + \Omega_2 b_e^\dagger(\mathbf{q})b_m(\mathbf{q}+\mathbf{k}_1) + \sqrt{N}\Omega_p b_e^\dagger(\mathbf{k}_p)b_g(0) + \text{H.c.}, \end{aligned} \tag{S3}$$

where $\Delta_p = \nu_p - \omega_{eg}$ is the detuning of the probe field which has frequency $\nu_p$, $\Delta_{2\text{ph}} = \nu_p - \nu_c - \omega_{mg}$ is the two-photon detuning. A source term $\Omega_p b_e^\dagger(\mathbf{k}_p)b_g(0)$ loads atoms from zero momentum ground state (BEC state) to the $|e\rangle$ state with $k_p$ momentum. The excitations are further transported via the coupling fields to $|m_l\rangle$ and $|e_l\rangle$ ($l$ is an integer). Since most of the atoms are in the BEC ground state, we can rewrite the Hamiltonian as

$$H = H_k + H_0 + H_{\rm NN} + H_{\rm source},$$

$$H_k = \sum_l \frac{\hbar^2(\mathbf{k}_p + 2l\mathbf{k}_1)^2}{2m} |e_l\rangle\langle e_l| + \frac{\hbar^2(\mathbf{k}_p + (2l-1)\mathbf{k}_1)^2}{2m} |m_l\rangle\langle m_l|, \tag{S4}$$

$$H_0 = \sum_l -\Delta_p |e_l\rangle\langle e_l| - \Delta_{\rm 2ph} |m_l\rangle\langle m_l, | \tag{S5}$$

$$H_{\rm NN} = \sum_n (\Omega_1 |e_l\rangle\langle m_l| + \Omega_2 |e_{l-1}\rangle\langle m_l|) + \text{H.c.}, \tag{S6}$$

$$H_{\rm source} = \sqrt{N}\Omega_p |e_0\rangle\langle N|_g + \text{H.c.}, \tag{S7}$$

where $H_0$ is the on-site energy of the states in superradiance lattice [S5], $H_{\rm NN}$ contains the nearest neighboring (NN) terms and $H_{\rm source}$ loads atoms from ground state $|N\rangle_g$ to the BEC timed-Dicke state $|e_0\rangle$ [S9]

For a weak probe field, we assume the steady state is $|\phi_s\rangle = |N\rangle_g + \sum_l A_l |e_l\rangle + B_l |m_l\rangle - O(A^2) - O(B^2)$, where $|A_n|(|B_n|) \ll 1$. The density matrix can be assumed as $\rho_s = |N\rangle_g \langle N|_g + (\sum_l A_l |e_l\rangle\langle N|_g + B_l |m_l\rangle\langle N|_g) + h.c.$ which satisfies the Liouville equation,

$$i\frac{\partial}{\partial t}\rho_s = [H, \rho_s] + \mathcal{L}(\rho_s), \tag{S8}$$

where $\mathcal{L}$ is the Lindblad superoperator. In the steady state, $\frac{\partial}{\partial t}\rho_s = 0$, which results in

$$\begin{pmatrix} ... & \Omega_2 & & & & \\ \Omega_2 & -\Delta_{\rm 2ph} & \Omega_1 & & & \\ & \Omega_1 & -\Delta_p - i\Gamma & \Omega_2 & & \\ & & \Omega_2 & -\Delta_{\rm 2ph} & \Omega_1 & \\ & & & \Omega_1 & -\Delta_p - i\Gamma & \Omega_2 \\ & & & & \Omega_2 & ... \end{pmatrix} \cdot \begin{pmatrix} ... \\ B_{-1} \\ A_0 \\ B_0 \\ A_1 \\ ... \end{pmatrix} = \begin{pmatrix} ... \\ 0 \\ \Omega_p \\ 0 \\ 0 \\ ... \end{pmatrix}, \tag{S9}$$

where $\Gamma = \gamma/2$ is the decoherence rate between $|e\rangle$ and $|g\rangle$. This equation can be solved numerically with a reasonable cutoff of its dimension. The solution of $A_l$ and $B_l$ are going to be used in the coupled-wave equations, as shown in the following.

## COUPLED-WAVE EQUATIONS

In the slowly-varying envelope approximation, the electric field and polarization of the atoms can be assumed as,

$$\mathbf{E}(t,z) = e^{i\mathbf{k}_p\cdot\mathbf{r} - iv_p t} E_+(z) + e^{i\mathbf{k}_b\cdot\mathbf{r} - iv_p t} E_-(z), \tag{S10}$$

$$\mathbf{P}(t,z) = e^{i\mathbf{k}_p\cdot\mathbf{r} - iv_p t} \epsilon_0 \chi_+ E_+(z) + e^{i\mathbf{k}_b\cdot\mathbf{r} - iv_p t} \epsilon_0 \chi_- E_-(z), \tag{S11}$$

where $E_+$ and $E_-$ are the probe and superradiance signal. The polarization of the atoms can be calculated as

$$\begin{aligned} \mathbf{P} &= \text{Tr}[e\hat{\mathbf{r}}\rho] \\ &= \langle\psi_s| \int d\mathbf{r}(\mu^* |\mathbf{r}\rangle_e \langle\mathbf{r}|_g + \mu |\mathbf{r}\rangle_g \langle\mathbf{r}|_e) |\psi_s\rangle \\ &= \langle\psi_s| \int d\mathbf{r}(\mu^* b_e^\dagger(\mathbf{r}) + \mu b_e(\mathbf{r})) |\psi_s\rangle, \end{aligned} \tag{S12}$$

In the Schrodinger picture, we decompose the positive and negative frequency components [S10]

$$\mathbf{P} \ = \ \frac{\mu}{\sqrt{2\pi}}\int d\mathbf{r}\sum_n A_n e^{i(\mathbf{k}_p+n(\mathbf{k}_1-\mathbf{k}_2))\cdot\mathbf{r}-iv_pt}. \tag{S13}$$

Since the atoms are homogeneously distributed, the polarization density can be written as

$$\mathbf{P}(x,t) = \frac{N}{V}\frac{\mu}{\sqrt{2\pi}}\sum_n A_n e^{i(\mathbf{k}_p+n(\mathbf{k}_1-\mathbf{k}_2))\cdot\mathbf{r}-iv_pt}. \tag{S14}$$

The polarizability of the probe field is

$$\begin{aligned}\chi_+ &= \frac{\mathbf{P}(x,t)}{\epsilon_0 E_+ e^{i\mathbf{k}_p\cdot\mathbf{r}-iv_pt}} \\ &= \frac{N\mu^2}{V\epsilon_0\hbar}\sum_n \tilde{A}_n e^{in(\mathbf{k}_1-\mathbf{k}_2)\cdot\mathbf{r}} &\text{(S15)} \\ &= \frac{3}{8\pi^2}\mathcal{N}\gamma\sum_n \tilde{A}_n e^{in(\mathbf{k}_1-\mathbf{k}_2)\cdot\mathbf{r}}, &\text{(S16)}\end{aligned}$$

where $\gamma = \frac{1}{4\pi\epsilon_0}\frac{4\omega^3\mu^2}{3\hbar c^3} = \frac{1}{3\pi\epsilon_0}\frac{\mu^2}{\hbar(\lambda/2\pi)^3}$ is the spontaneous decay rate and $\mathcal{N} = \frac{N}{V}\lambda^3$, i.e., the atom number in a cubic wavelength. We adopt a two-mode approximation, i.e., only the probe field and the superradiant field from the state $|e_n\rangle$ is considered in the coupled-wave equation. The relevant components in the polarizability are

$$\begin{aligned}\chi_+ &= \chi_0 + \chi_{-2n}e^{-in(\mathbf{k}_1-\mathbf{k}_2)\cdot\mathbf{r}} = \frac{3}{8\pi^2}\mathcal{N}(\tilde{A}_0 + \tilde{A}_{-n}e^{-i2nk_1\sin\theta/2x}), &\text{(S17)} \\ \chi_- &= \chi_0 + \chi_{2n}e^{in(\mathbf{k}_1-\mathbf{k}_2)\cdot\mathbf{r}} = \frac{3}{8\pi^2}\mathcal{N}(\tilde{A}_0 + \tilde{A}_n e^{i2nk_1\sin\theta/2x}). &\text{(S18)}\end{aligned}$$

The coupled-wave equation is

$$\frac{\partial}{\partial x}E_+ = -\beta_0 E_+ + i\kappa_{2n}e^{-i\Delta kx}E_-, \tag{S19}$$

$$\frac{\partial}{\partial x}E_- = \beta_0 E_- - i\kappa_{-2n}e^{i\Delta kx}E_+, \tag{S20}$$

where $\beta = \beta_0 - i\Delta k/2$, $\beta_0 = \frac{v_p^2}{(1+\sin\frac{\theta}{2})k_pc^2}\mathrm{Im}\chi_0$ and $\kappa_{\pm 2n} = \frac{v_p^2}{(1+\sin\frac{\theta}{2})k_pc^2}\chi_{\pm 2n}$. With the boundary conditions $E_+(0) = E_0$ and $E_-(L) = 0$, we obtain

$$R = \left|\frac{\kappa_{-2n}(e^{-\lambda L} - e^{\lambda L})}{(\beta-\lambda)e^{-\lambda L} - (\beta+\lambda)e^{\lambda L}}\right|^2, \tag{S21}$$

$$T = \left|\frac{2\lambda}{(\beta-\lambda)e^{-\lambda L} - (\beta+\lambda)e^{\lambda L}}\right|^2, \tag{S22}$$

where $\lambda = \sqrt{\beta^2 + \kappa_{2n}\kappa_{-2n}}$.

## BEC AND NON-CONDENSED ATOMS

Although in theory BEC atoms and cold atoms have no difference, the spectra we measured shows that experimentally cold atoms have other complications. In the original proposal [S5] the authors assumed that the atoms are uniformly excited by the probe field such that a timed Dicke state with equal excitation probabilities for each atom can be prepared. With this assumption no difference exists for condensed and non-condensed atoms. However, it is hard to achieve a uniform excitation of non-condensed atoms in experiments. How to make the sample optically thin

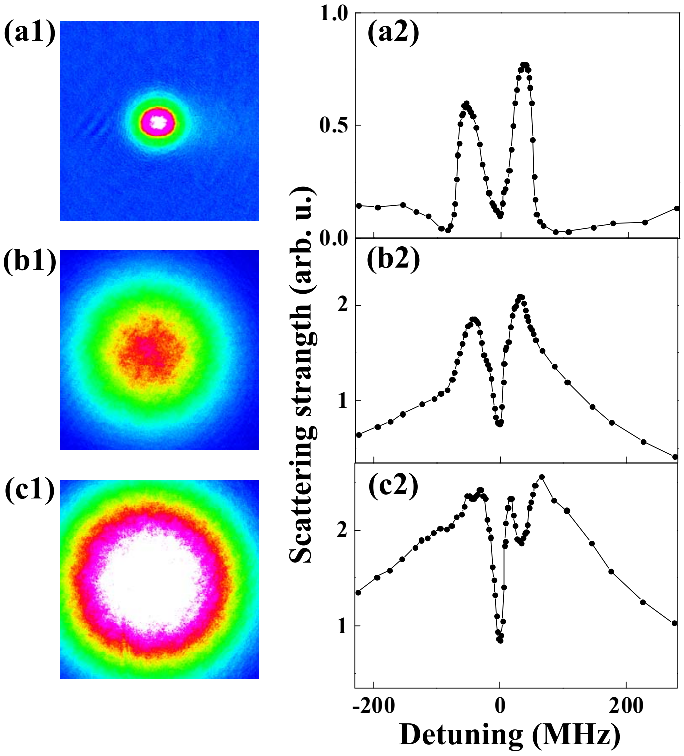


FIG. S4: **Comparison between the reflection spectra of BEC atoms and cold atoms at different temperatures.** (a1) The time of flight (TOF) absorption image of BEC free expansion time $\tau$ =30 ms. (a2) The superradiant spectra for BEC. (b1) The TOF image of cold atoms at temperature $T = 10\ \mu K$ with $\tau$ =15 ms. (b2) The superradiant spectra for cold atoms in (b1). (c1) The TOF image of cold atoms at temperature $T = 24\ \mu K$ with $\tau$ =15 ms. (c2) The superradiant spectra for cold atoms in (c1).

in absorption and optically thick in emission has been extensively discussed in theory [S12] and realized only with delicate design in experiments [S13]. With cold atoms in general, the atoms at the entrance of the sample have a larger chance to be excited, i.e., the atoms are non-uniformly excited, which results in excitation of many subradiant states and brings complications in the spectra. In contrast, a BEC with all atoms sharing the same ground state wavefunction and a smaller size can be much more uniformly excited across the sample, which provides an ideal situation for investigating superradiance and collective Lamb shift. In Fig. S4, we compare the superradiant spectra in both BEC atoms and cold atoms at different temperatures. It is easily seen that only the BEC spectrum has a reasonable width that can be explained by the superradiance lattice, in particular for the left peak.

## ATOMIC DENSITY MODULATION

Similar reflection [S14] and blue-red asymmetry [S15] has been observed and attributed to the atomic density modulation. In order to clarify the difference between our results and the previous references, we first compare the parameters. The potential depth of the optical lattice induced by the coupling field in our experiment is $\Omega_1^2/6.9$GHz $\simeq 0.06$ MHz (standing wave intensity 40 mW/cm$^2$). In Ref. [S14], according to $U/k_BT = 3.5$, the potential depth is around 7 MHz. In Ref. [S15], the potential depth is $\Omega^2/5.89$MHz $\simeq 10^2$ MHz (standing wave intensity 20 mW/cm$^2$). We notice that our potential depth is much shallower than the previous two works. In addition, the waiting time for the atoms to reach a thermal equilibrium in Ref. [S14] is a few ms, whereas in our case, the interaction time is only 10 $\mu s$. The density modulation is much weaker than these previous works.

It is difficult to measure the density modulation of the sample. To obtain experimental evidence that the density modulation is not the reason of the observed results, we measured the reflection spectra of BEC atoms with only density modulation. We use a pair of strong coupling laser beams with the wavelength near 780 nm. In this case the standing wave serves as an optical lattice of the atoms (similar to Ref. [S14] but in BEC atoms). The reflection

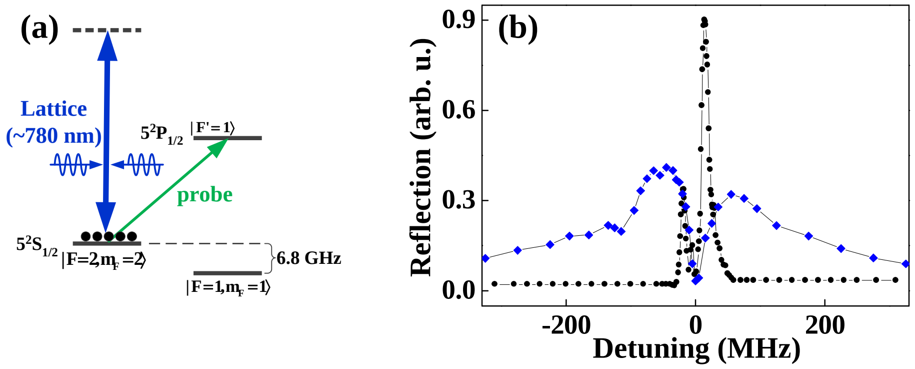


FIG. S5: **Comparison of the reflection spectra of the superradiance lattice and the density modulated sample.**(a) Energy levels and laser detuning for a density modulated BEC sample. A pair of strong coupling laser beams have the wavelength near 780 nm. (b) The reflection spectra due to the density modulation (blue diamonds) and the superradiance lattice (black circles). For the superradiance lattice, $\Delta_c = 0$.

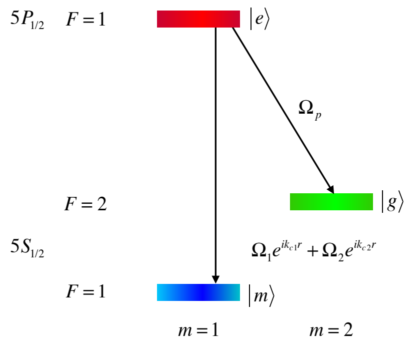


FIG. S6: Atomic level scheme used in theoretical fitting.

spectrum is shown as the blue diamonds in Fig. S5, which is very different from that of the superradiance lattice (black circles). First of all, the spectrum is much wider. The width of the spectrum is not directly related to the Rabi frequency of the coupling field, while in superradiance lattice the width of the spectrum is four times the Rabi frequency and the spectrum has a sharp cutoff at the ends. This can be easily understood since superradiance is an on-resonance radiative phenomenon such that the frequency of the probe field must lie in the energy band of the lattice, while photonic crystal due to the periodic modulation of the dispersion allows the probe field to be far off-resonance. In addition, the relative strengths of the two peaks are reversed, which is a combinational effect of phase matching with different dispersion and collective interaction.

## NUMERICAL SIMULATION

In the theoretical fitting, the effective atomic density is $N = 10^{19}\ m^{-3}$ (which is slightly less than experimental typical density due to the heating effect of lattice fields), the effective sample length is 16 periods of the standing wave pattern, the Rabi frequency of the probe field is $\Omega_p = 1.5$ MHz, and the decoherence rate is 2 MHz. In Fig. 3(a1)-(a4) of the main text, the Rabi frequencies of the coupling fields are $\Omega_1 = \Omega_2 = \Omega = 5$ MHz, 8 MHz, 11 MHz, 16 MHz from top to bottom. The detuning of the lattice fields is $\Delta_c = 0$ MHz, and the wave vector mismatch is $\Delta k = 0$. In Fig. 3 (b1)-(b4) of the main text, the detunings of the lattice fields are $\Delta_c = -10$, 0 MHz, 10 MHz, 20 MHz from top to bottom. The Rabi frequency of the lattice fields is $\Omega = 11$ MHz, and the wave vector mismatch is $\Delta k = 0$. In Fig. 4(a)-(e) of main text, the wave vector mismatch is $\Delta k = -0.02 \times 2\pi/\lambda$, $0.01 \times 2\pi/\lambda$, $0.02 \times 2\pi/\lambda$ , $0.03 \times 2\pi/\lambda$, and $0.04 \times 2\pi/\lambda$ from top to bottom. The Rabi frequency of the lattice field is $\Omega = 11$ MHz, and the detuning of the lattice fields is $\Delta_c = 0$ MHz. The atomic level scheme is plotted in Fig. S6. One remark is that the EIT condition fails at the nodes of the standing wave since the coupling field is stronger than the probe field. Therefore we need to

consider the population redistribution on the state $|m\rangle$.

The two peaks in most of the figures are asymmetric. Part of the asymmetry can be attributed to the phase mismatch $\Delta k$. The finite size $L$ of the BEC brings a finite resolution of the momentum, $\delta k = 2\pi/L$. For an infinitely long BEC, the phase matching is achieved in a unique direction. On the other hand, if the BEC is much smaller than the wavelength of the light, there is no preferred direction of the superradiant emission. In our experiment, within the size of the BEC there are around 16 periods of the standing wave. Instead of determining the position of a reflection band with near unity reflectance around the phase matching point for a much longer sample, the dispersion only introduces a slight bias between the heights of the two reflection peaks, similar to the optical Bragg scattering experiment of cold atomic gases in optical lattices.

The major discrepancy between the experimental data and the theoretical fitting is that the peak widths increase and the spectra shifts to the red side further than predicted when the power of the coupling field increases. The two inconsistencies may be attributed to the collective decay rate and Lamb shift, as well as the non-zero momentum component in the BEC.

*pengjun_wang@sxu.edu.cn.
†hcai@tamu.edu.
‡jzhang74@sxu.edu.cn, jzhang74@yahoo.com.

[S1] H. M. Price, T. Ozawa, and I. Carusotto, Phys. Rev. Lett. **113** (2014).
[S2] P. Wang, Z.-Q. Yu, Z. Fu, J. Miao, L. Huang, S. Chai, H. Zhai, and J. Zhang, Phys. Rev. Lett. **109** (2012).
[S3] L. W. Cheuk, A. T. Sommer, Z. Hadzibabic, T. Yefsah, W. S. Bakr, and M. W. Zwierlein, Phys. Rev. Lett. **109** (2012).
[S4] M. B. Dahan, E. Peik, J. Reichel, Y. Castin, and C. Salomon, Phys. Rev. Lett. **76**, 4508 (1996).
[S5] D.-W. Wang, R.-B. Liu, S.-Y. Zhu, and M. O. Scully, Phys. Rev. Lett. **114**, 043602 (2015).
[S6] A. Polkovnikov, S. Sachdev, and S. M. Girvin, Phys. Rev. A **66** (2002).
[S7] C. Hooley and J. Quintanilla, Phys. Rev. Lett. **93** (2004).
[S8] Y.-J. Lin, K. Jiménez-García, and I. B. Spielman, Nature **471**, 83 (2011).
[S9] M. O. Scully, E. S. Fry, C. H. R. Ooi, and K. Wódkiewicz, Phys. Rev. Lett. **96**, 010501 (2006).
[S10] A. André and M. D. Lukin, Phys. Rev. Lett. **89**, 143602 (2002).
[S11] D. W. Wang, H. T. Zhou, M. J. Guo, J. X. Zhang, J. Evers, and S. Y. Zhu, Phys. Rev. Lett. **110**, 093901 (2013).
[S12] B. W. Adams, J. Mod. Opt. **56**, 1974 (2009).
[S13] R. Rohlsberger, K. Schlage, B. Sahoo, S. Couet, Sebastien R. Rffer, Science **328**, 1248 (2010).
[S14] A. Schilke, C. Zimmermann, P. W. Courteille, and W. Guerin, Phys. Rev. Lett. **106**, 223903 (2011).
[S15] G. L. Gattobigio, F. Michaud, J. Javaloyes, J. W. R. Yabosa, and R. Kaiser, Phys. Rev. A **74**, 043407 (2006).
